# Supplementary material for: Spin-dimer ground state driven by consecutive charge and orbital ordering transitions in the anionic mixed-valence compound Rb$_4$O$_6$
Source: arXiv:1911.12049 source file (2019-11-27)
Supplement: Supplementary file 1 [file Rb4O6-SM2.pdf]

# Spin-dimer ground state driven by consecutive charge and orbital ordering transitions in the anionic mixed-valence compound $Rb_4O_6$

## Supplemental information

T. Knaflič,[1] P. Jeglič,[1] M. Komelj,[1] A. Zorko,[1, 2] P. K. Biswas,[3] A. N. Ponomaryov,[4] S. A. Zvyagin,[4] M. Reehuis,[5] A. Hoser,[5] M. Geiß,[6] J. Janek,[6] P. Adler,[7,*] C. Felser,[7] M. Jansen,[7,#] and D. Arčon[1, 2,§]

[1]Jožef Stefan Institute, Jamova c. 39, 1000 Ljubljana, Slovenia
[2]Faculty of Mathematics and Physics, University of Ljubljana, Jadranska c. 19, 1000 Ljubljana, Slovenia
[3]ISIS Pulsed Neutron and Muon Source, STFC Rutherford Appleton Laboratory, Didcot OX11 0QX, UK
[4]Dresden High Magnetic Field Laboratory (HLD-EMFL), Helmholtz-Zentrum Dresden-Rossendorf, 01328 Dresden, Germany
[5]Helmholtz-Zentrum Berlin für Materialien und Energie, 14109 Berlin, Germany
[6]Institute of Physical Chemistry and Center for Materials Research, Justus-Liebig- University Giessen, Heinrich-Buff-Ring 17, 35392 Giessen, Germany
[7]Max Planck Institute for Chemical Physics of Solids, Nöthnitzer Straße 40, 01187 Dresden, Germany

[*] adler@cpfs.mpg.de
[#] m.jansen@fkf.mpg.de
[§] denis.arcon@ijs.si

## Refinement of high-resolution powder neutron diffraction patterns

Powder neutron diffraction (PND) investigation show that $Rb_4O_6$ undergoes a structural transition from the cubic (space group $I\bar{4}3d$, No. 220) to the tetragonal (space group $I\bar{4}$, No. 82) crystal structure. Structural transition starts at around $T$ = 290 K and is nearly completed at $T$ = 250 K. The temperature dependence of the fractions of the cubic and tetragonal phase in the slow cooling mode is derived from the Rietveld refinements of data collected on instrument E6 at the BER II reactor of the Helmholtz-Zentrum Berlin and is shown in Fig. S1.

The results of the Rietveld refinements of the data collected at instrument E9 are shown in Fig. S2. The high-temperature cubic crystal structure of $Rb_4O_6$ was refined in the space group $I\bar{4}3d$ (No. 220). For the Rietveld refinements of the PND pattern collected at 400 K, we have used the values from the x-ray data of cubic $Rb_4O_6$ (Ref. [29] in the main text) as starting values. In this setting the Rb and O atoms are located at the Wyckoff position 16$c$($x$,$x$,$x$) and 24$d$($x$',0,¼) [in our case ($x$,0,¾) with $x$ = ½ – $x$'], respectively. The refinement of the positional parameters $x$(Rb) and $x$(O) as well as of the two thermal parameters resulted in a somewhat enlarged residual $R_F$ = 0.106 (defined as $R_F = \Sigma\,||F_{\mathrm{obs}}| - |F_{\mathrm{calc}}||/\,\Sigma|F_{\mathrm{obs}}|$). This can be ascribed to the fact that the strongly enlarged thermal parameters lead to a strong continuous decrease of the intensity of Bragg reflections up to

higher scattering angles as it can be seen in Fig. S2, top. However, the positional and thermal parameters could be determined to a good accuracy. For the data set collected at 100 K a much smaller residual $R_F$ = 0.043 was obtained, because of the much higher intensity of the high-order Bragg reflections (Fig. S2, bottom). At this temperature the crystal structure of the dominating tetragonal phase of $Rb_4O_6$ was refined in the space group $I\bar{4}$ (No. 82). The two crystallographically distinct atoms Rb1 and Rb2 occupy the Wyckoff positions 8*g*(*x*,*y*,*z*), while the O atoms are located at the following positions: O1 at 4*e*(0,0,*z*), O2 at 4*f*(0,½,*z*) and both O3 and O4 at 8*g*(*x*,*y*,*z*). In the refinements we have considered the two types of anions ($O_2^{2-}$ and $O_2^-$ as rigid groups, where a soft constraint was applied by setting a standard deviation of the ideal value of the bond distance *d* (in our case a ratio of $\sigma/d$ = 0.001). For the peroxide and superoxide anions, $O_2^{2-}$ (atoms labeled as O1 and O2) and $O_2^-$ (atoms labeled as O3 and O4), we have obtained the bond distances 1.524(4) and 1.312(7) Å, which are slightly smaller than the ideal values of 1.54 and 1.33 Å, respectively. At 2.9 K additional Bragg reflections were found obeying the extinction rule $h + k + l = 2n + 1$. This clearly suggests the loss of the *I*-centered symmetry. Therefore, we carried out the crystal-structure refinements in the next-lower symmetric space group $P\bar{4}$ (No. 81) which resulted in a satisfactory residual $R_F$ = 0.041. In this space group each atom site splits into the following Wyckoff positions: two sites 4*h*((*x*,*y*,*z*) for O3, O4 and all Rb atoms; 2*e*(0,0,*z*) and 2*f*(½,½,*z*) for O1; two sites 2*g*(0,½,*z*) for O2.

In the cubic phase one only finds one single bond length for the $O_2$ units. Due to the fact that the concentration ratio of the $O_2^-$ and $O_2^{2-}$ anions is exactly two the average charge of the $O_2$ units is −4/3. Therefore, we expect an average bond length of 1.40 Å. From our unrestricted refinements we have obtained a reduced bond length of 1.256(3) Å at 400 K. Accordingly, in the refinement, similar as in the refinement of the tetragonal structure, a constraint was used and an ideal O-O bond length of 1.40 Å was taken as starting value. Finally, bond lengths of 1.350(4) Å were obtained. It has to be mentioned that the residual $R_F$ of the cubic structure was slightly increased from 0.103 to 0.106 by using this constraint. On the other hand, the residual $R_F$ = 0.043 for the tetragonal structure remained practically unchanged. The results of the refinements are summarized in Tables S1 and S2 as well as in Fig S2.

In a control PND experiment run at instrument E6 ($\lambda$ = 2.426 Å), we have applied a rapid cooling procedure: the $Rb_4O_6$ sample was quenched into liquid nitrogen from 400 down to 80 K with an average cooling rate of about 40 K per minute. Then it was further cooled down to 3 K in the cryostat with a cooling rate of 2-3 K per minute. The pattern collected at 2 K matches (Fig. S3) the cubic structure, which is thus almost completely frozen-in in such quench cooling experiments.

## Impact of different cooling protocols

In measurements of the static molar susceptibility, $\chi_m(T)$, we tested the influence of different cooling protocols on the magnetic properties (Fig. S5). In the slow cooling experiment, a cooling rate of 2 K/ min was applied starting from 400 K, while in the rapid cooling procedure a cooling rate of 20 K/min was applied.

In continuous wave X-band electron paramagnetic resonance (EPR) experiments, we always found a residual signal at low temperatures (Fig. S6), that is markedly different from the much broader EPR signal of the tetragonal phase (Fig. 5 in the main text). This signal can be fitted to a lineshape with *g*-factor anisotropy. The fit converged to the axially-symmetric g-factor anisotropy yielding $g_x = g_y = 1.9757$ and $g_z = 2.3110$ and a small Lorentzian broadening of $\Delta B_x = \Delta B_y = 29.2$ mT and $\Delta B_z = 33.3$ mT. In the lineshape fitting procedure a broad background signal was added with $g = 2.0242$ and $\Delta B = 247$ mT.

## X band EPR measurements

*Quench experiment*

The $Rb_4O_6$ powder sample (the same one as used in all other EPR experiments), was in these set of experiments first heated to 400 K for an extended period in order to ensure 100% cubic phase. The sample was then directly submerged into liquid nitrogen and was after thermalization quickly transferred into a pre-cooled EPR He-flow cryostat at 100 K. The sample was then rapidly cooled down to base temperature of 3.4 K in several minutes. The X band EPR measurements were then conducted on heating. According to powder neutron diffraction results (Fig. S3), such thermal protocol ensures that the cubic phase is completely frozen in at low temperatures. With increasing temperature, the cubic phase remains metastable up to 160 K, where the tetragonal phase starts to appear.

X-band EPR spectra of the quenched cubic phase appear as a very broad Lorentzian line with a linewidth of 830 mT at 3.4 K (Fig. S7). With increasing temperature, the EPR spectra become even broader, while the EPR signal intensity decreases (Fig. S8). The EPR signal intensity follows the Curie-Weiss law with a small Curie temperature (inset to Fig. S8). Above ~ 50 K the spectral linewidth exceeds 1 T and as a result measurements of EPR spectra become difficult. The broadening trend continues and together with decreasing intensity, we could extract at best only rough estimates of spectral parameters. However, above 157 K the X-band EPR signal suddenly reappears [Fig. S7(c)], marking the transition from the metastable cubic to the tetragonal phase. The reappearance of tetragonal EPR signal above 157 K thus corroborates the powder neutron diffraction data (Fig. 2 (b), main text). Above 157 K, the linewidth and the *g*-factor of the EPR spectra follow again the trend from the measurements of the tetragonal phase taken during the slow-cooling experiments (main text).

## Impedance spectroscopy and transport data

$Rb_4O_6$ pellets with a diameter of 6 mm and a thickness of around 1 mm were pressed for impedance measurements. Gold foil with a diameter of 6 mm as electrodes was fixed to the two sides of the $Rb_4O_6$ pellets. The pellets were connected with nickel tabs as current collectors and were sealed in gas-tight pouch foil in an argon-filled glovebox [MBRAUN, < 0.1 parts per million (ppm) $H_2O$, < 0.1 ppm $O_2$]. Temperature-dependent impedance measurements were then carried out using an Alpha-A mainframe by Novocontrol Technologies with an equipped POT/GAL30V2A electrochemical test station and a ZG4 test interface. The measurements were carried out in a temperature range of 373 K to 173 K in steps of 5 K. The temperature was adjusted using a liquid nitrogen–based cooling system and a heating coil. The sample holder was placed in a steel vessel, where it was cooled in the nitrogen gas flow. For each temperature step, a relaxation time of 2.5 hours was chosen with a maximum temperature change of 0.3 K/min. The impedance was measured between 10 MHz and 10 mHz with a sinus amplitude of 10 mV. Data evaluation was performed using the software RelaxIS 3 (rhd instruments). For fitting the data, an equivalent circuit consisting of a parallel resistor $R$ and a constant phase element $Q$ was chosen. From the resulting resistances, the electrode area and the thickness of the sample, temperature-dependent conductivities $\sigma_{el}$ were calculated. Due to the high resistance of the sample, conductivities at temperatures below 203 K could not be determined.

The impedance measurement can be used to derive further transport properties. Assuming a charge carrier density $n$ of $4/V_{\text{cell}}$ ($V_{\text{cell}}$ represents the unit cell calculated from the lattice parameters given in Fig. 2), the electron mobility $u$ as a function of temperature (Fig. S11) can be calculated from the electronic conductivity $\sigma_{\text{el}}$ as $u = \frac{\sigma_{\text{el}}}{e_0 \cdot n}$, with the electron charge $e_0$. Because the electron concentration changes only due to the thermal lattice expansion, the dramatic jump in conductivity directly represents a jump of the electron mobility. Using the Nernst-Einstein relation $D = \frac{u \cdot k_{\text{B}} \cdot T}{e_0}$, the diffusion coefficient $D$ can be retrieved from the mobility using the Boltzmann constant $k_{\text{B}}$ and the absolute temperature $T$ (Fig. S12).

Assuming isotropic diffusion of the electrons, the diffusion coefficient D is related to the jump distance $a$ and the jump frequency ω according to $D = 1/6 \cdot a^2 \cdot \omega$. For the jump distance, the shortest intermolecular distance between the oxygen dumbbells was used. This results in $a$ = 439 pm for the cubic structure and $a$ = 411 pm for the tetragonal structure, leading to the jump frequency in Fig. S13.

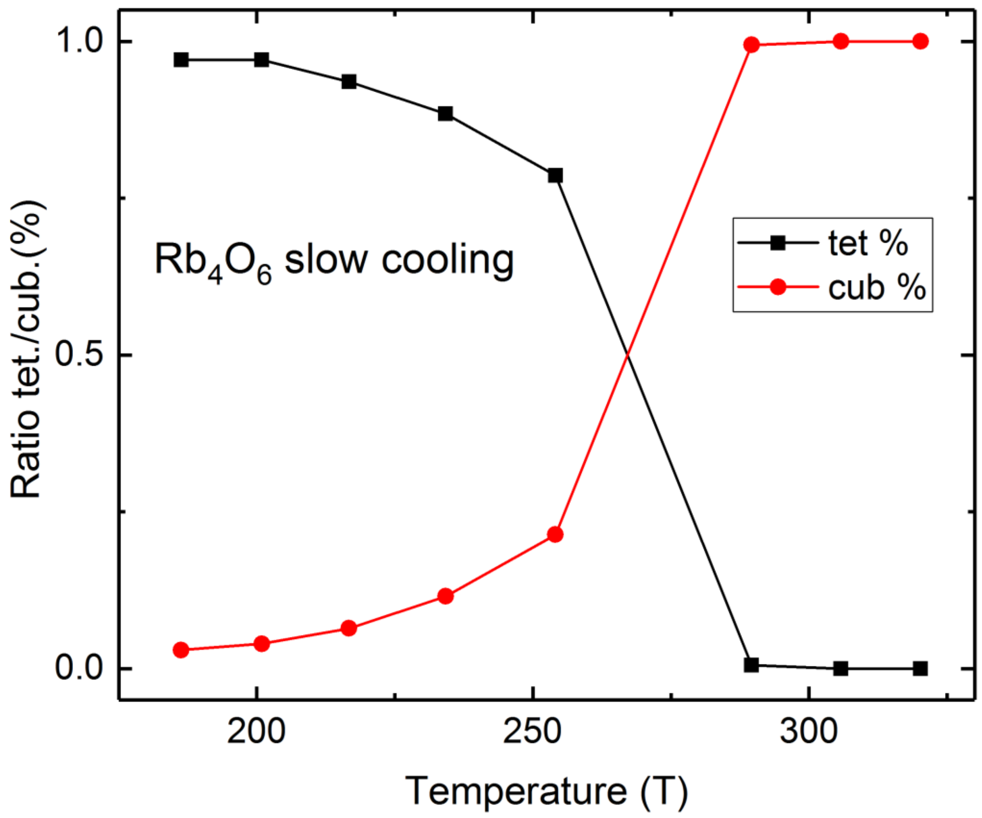


**FIG. S1** Temperature dependence of the fractions of the cubic and tetragonal phases in the slow cooling mode derived from the Rietveld refinements of data collected on instrument E6.

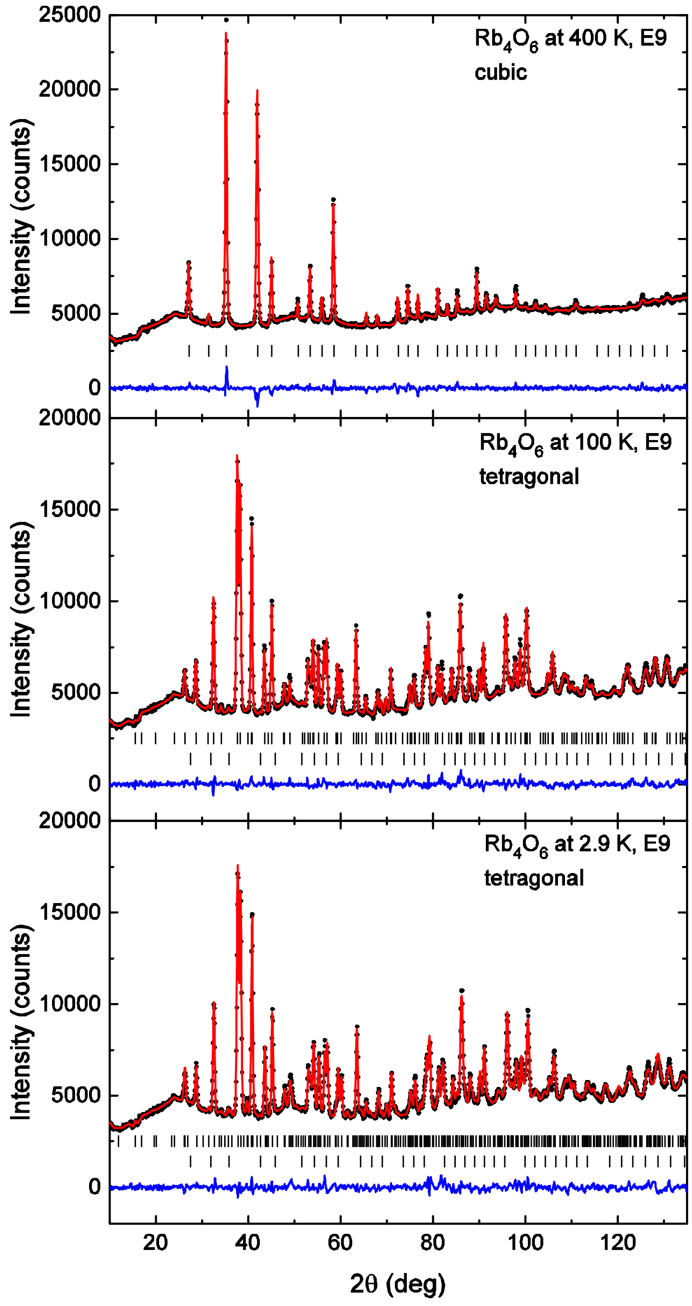


**FIG. S2** Powder neutron diffraction patterns of $Rb_4O_6$ collected at instrument E9 ($\lambda$ = 1.7985 Å). The pattern collected at 100 K was obtained after slow cooling which assured a nearly complete conversion to the tetragonal phase. At 2.9 K additional Bragg reflections were found obeying the extinction rule $h + k + l = 2n + 1$. The calculated pattern (red solid line) is compared with the observations (black-filled circles). The positions of the nuclear reflections (black bars) of the cubic and tetragonal phase, as well as the difference pattern ($I_{obs} - I_{cal}$) (blue solid line) is shown.

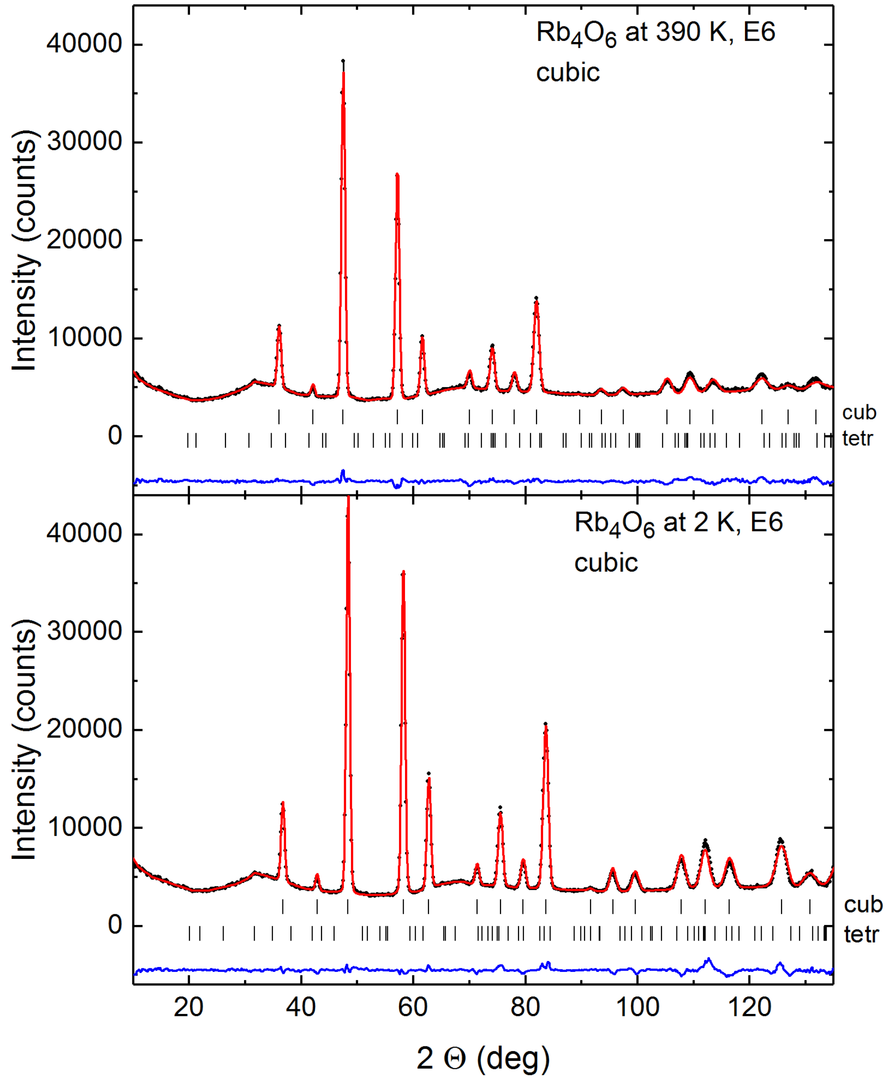


**FIG. S3** Powder neutron diffraction patterns of $Rb_4O_6$ collected at instrument E6 (λ = 2.426 Å). The pattern collected at 2 K was obtained after quenching into liquid nitrogen, which completely preserved the cubic phase. The calculated pattern (red solid line) is compared with the observations (black-filled circles). The positions of the nuclear reflections (black bars) of the cubic and tetragonal phase, as well as the difference pattern ($I_{obs} - I_{cal}$) (blue solid line) is shown.

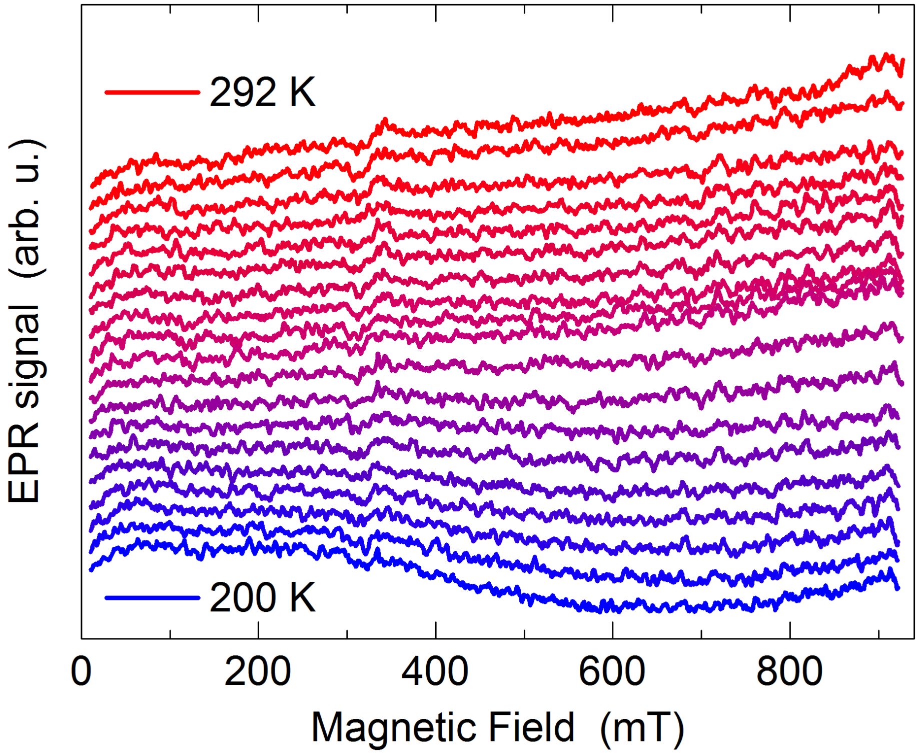


**FIG. S4** The structural transition from the cubic (red) to the tetragonal (blue) phase as seen by the emergence of the EPR signal. The spectra were measured in 5 K steps.

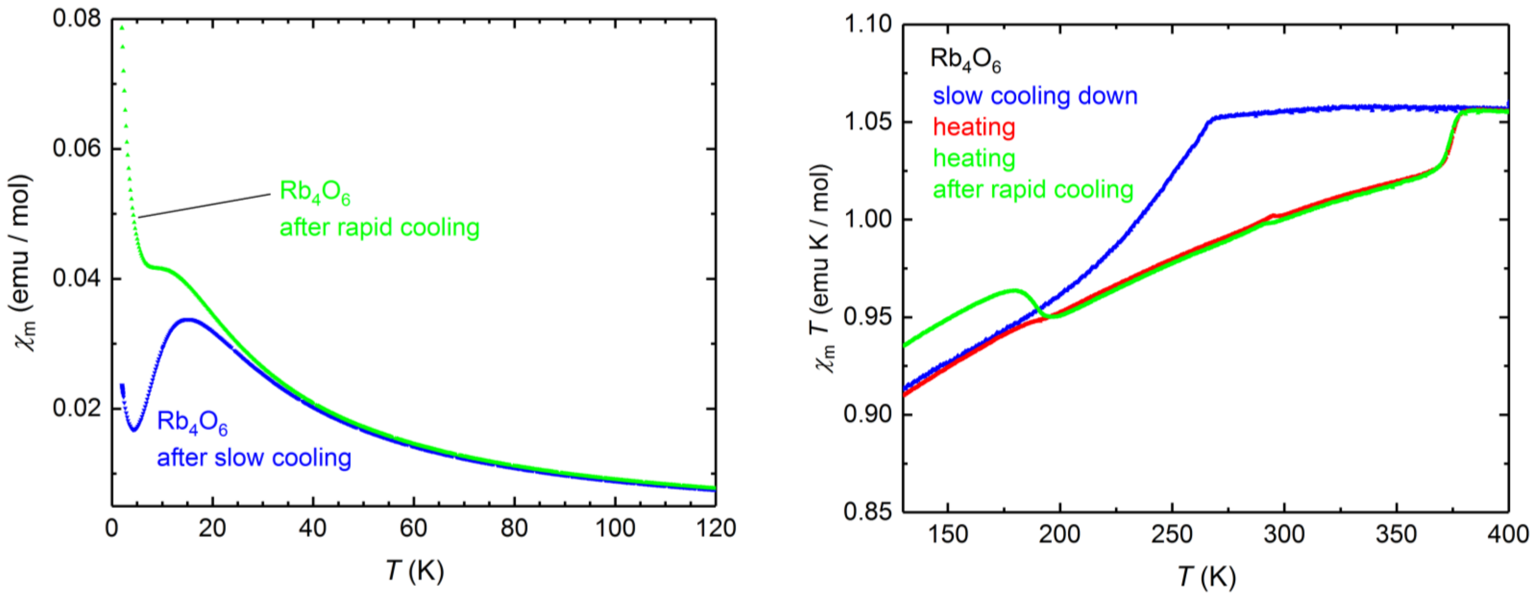


**FIG. S5** Measurements of molar susceptibility, $\chi_m(T)$, of $Rb_4O_6$ powder using different cooling protocols. In the slow cooling experiment a cooling rate of 2 K/ min was applied starting from 400 K, in the rapid cooling procedure a cooling rate of 20 K/min was applied. Left panel: Rapid cooling leads to an enhanced increased Curie tail in $\chi_m(T)$ at low temperatures which partly obscures the maximum associated with the tetragonal phase. This is a signature of an increased fraction of frozen-in cubic phase. Right: The frozen cubic phase is the origin for an anomaly near 180 K which reflects the transformation of the metastable cubic phase to the tetragonal phase. The reverse tetragonal to cubic transformation occurs near 370 K in both temperature protocols.

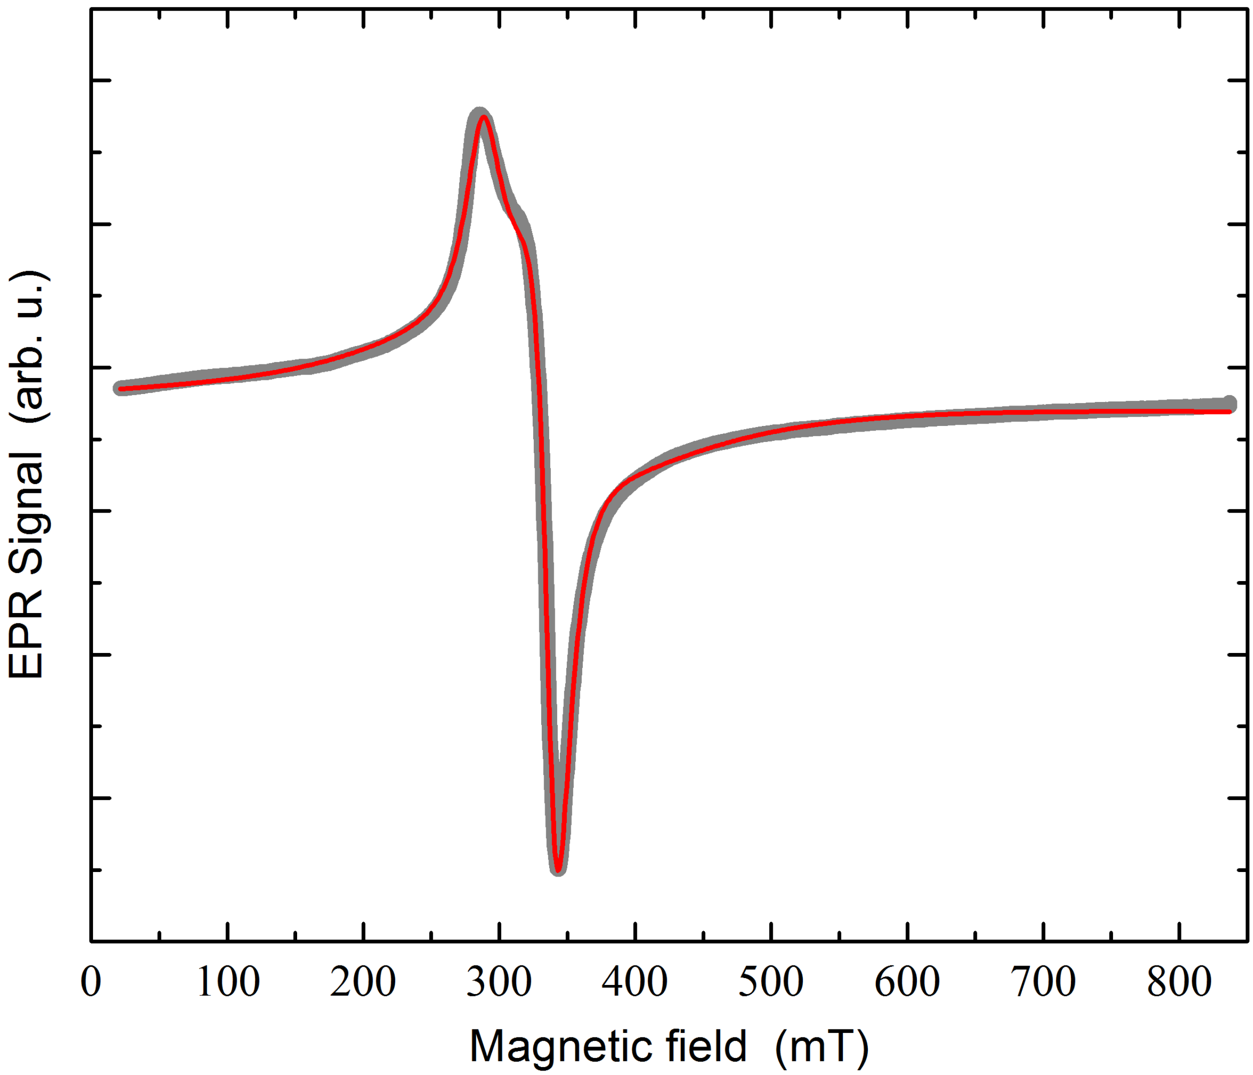


**FIG. S6** The residual X-band EPR spectrum measured at 3.5 K in the tetragonal phase (gray line). Red line is a fit to Lorentzian lineshape with added *g*-factor anisotropy, yielding $g_x = g_y =$ 1.9757, $g_z = 2.3110$, $\Delta B_x = \Delta B_y = 29.2$ mT and $\Delta B_z = 33.3$ mT.

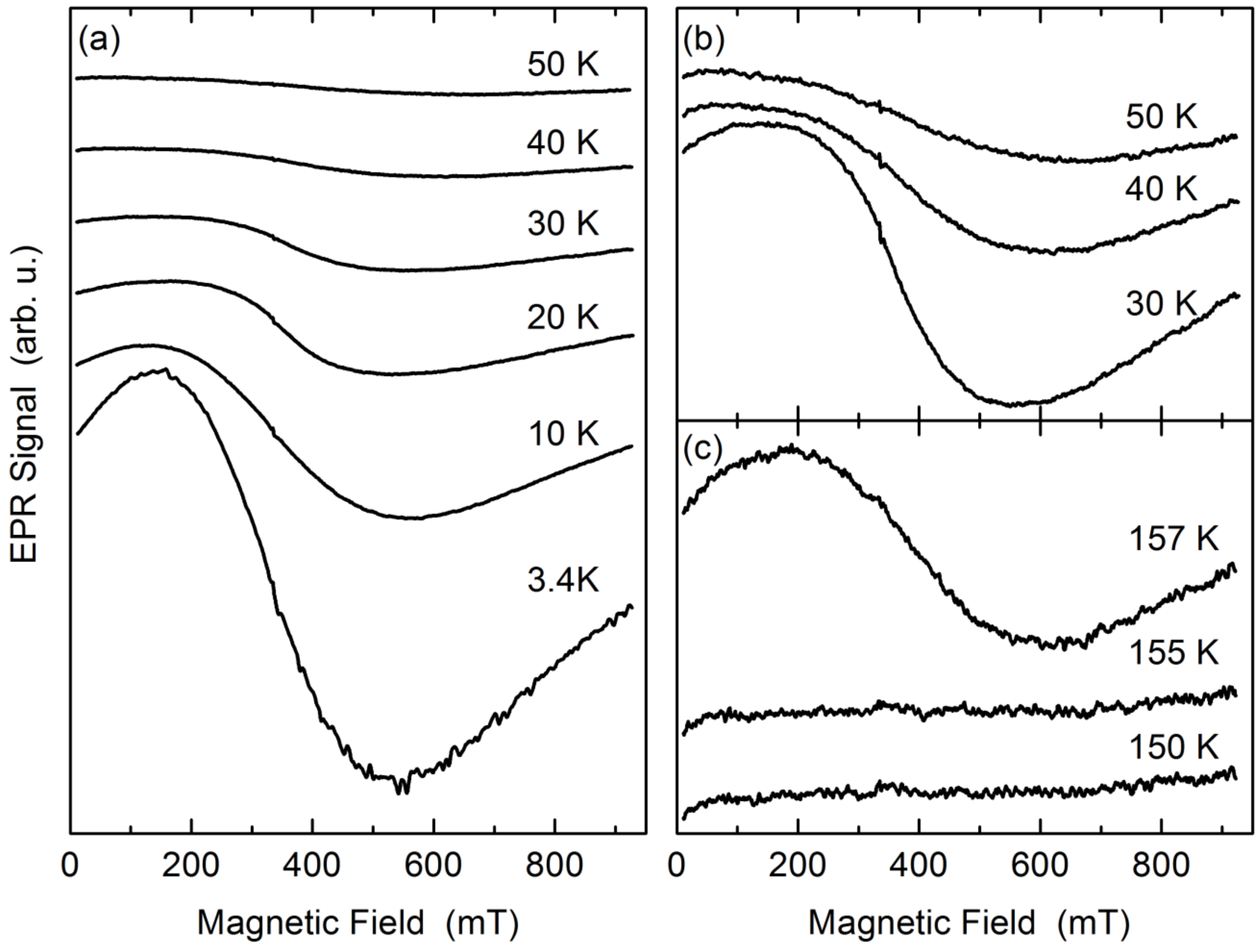


**FIG. S7** The X-band EPR spectra of the cubic phase in the quench experiment. (a) Temperature dependence of the EPR spectra after quenching the sample from 400 K at selected temperatures between 3.4 K and 50 K. The spectra have a large linewidth, which even increases with increasing temperature. The EPR signal intensity, on the other hand, decreases with increasing temperature. (b) Comparison of X-band EPR spectra collected at 30, 40 and 50 K show large spectral broadening. (c) X-band EPR spectra at higher temperatures, showing the reappearance of the EPR signal characteristic of the tetragonal phase. According to EPR, the tetragonal phase thus starts to grow from the quenched cubic phase above 157 K, which is in excellent agreement with the powder neutron diffraction results (Fig. 2(b), main text).

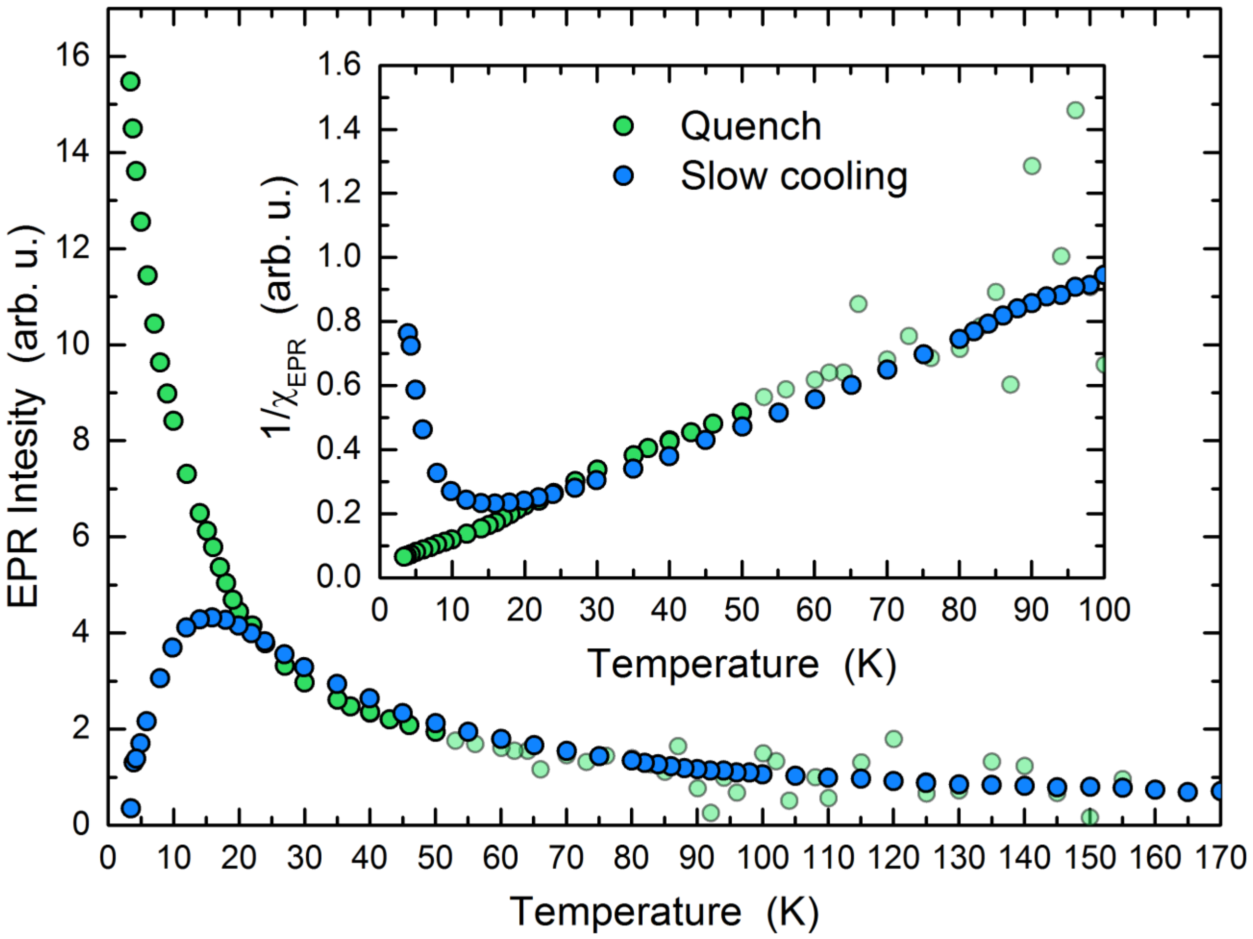


**FIG. S8** The X-band EPR signal intensity of cubic (green circles) and tetragonal (blue circles) phase. Also, the green and blue circles represent EPR measurements when quenching and slow-cooling of the sample were used, respectively. The inverse EPR signal intensity demonstrates the Curie-Weiss temperature dependence of the EPR signal intensity, which in the case of cubic phase persists down to 3.4 K.

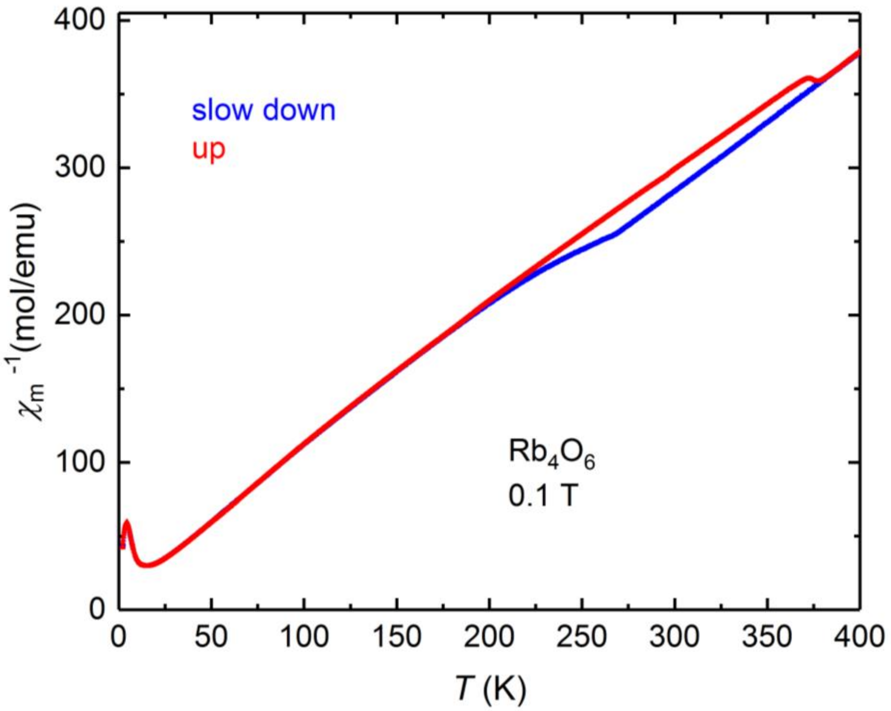


**FIG. S9** Curie-Weiss plot of the magnetic susceptibility data of $Rb_4O_6$ measured at 1 T after slow cooling to 2 K. The anomalies reflect the cubic – tetragonal – cubic structural transitions on cooling and subsequent heating. Using the temperature range 50 to 120 K one obtains the effective magnetic moment $\mu_{eff}$ = 1.95 $\mu_B$ and a Curie-Weiss temperature $\Theta$ = –7 K for the tetragonal phase. For the cubic phase one obtains $\mu_{eff}$ = 2.05 $\mu_B$ and $\Theta$ = +1 K for the temperature range from 320 to 400 K using the data from the cooling down protocol.

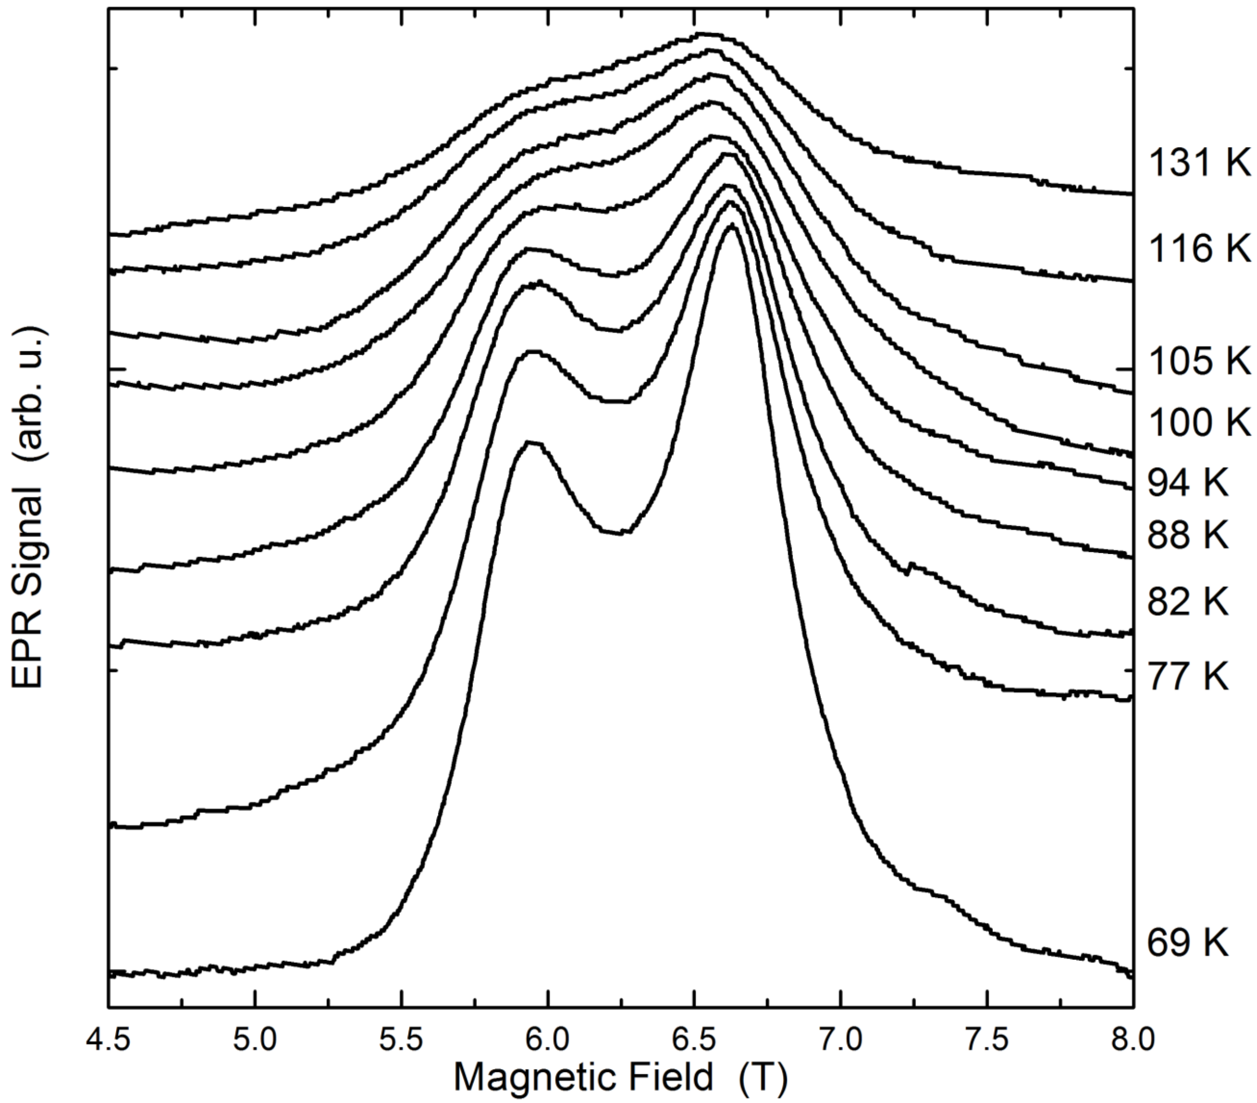


**FIG. S10** Temperature dependence of the high-field EPR spectra measured at 186 GHz on heating. The splitting of the spectra is clearly visible and gradually becomes less pronounced above $T_S$.

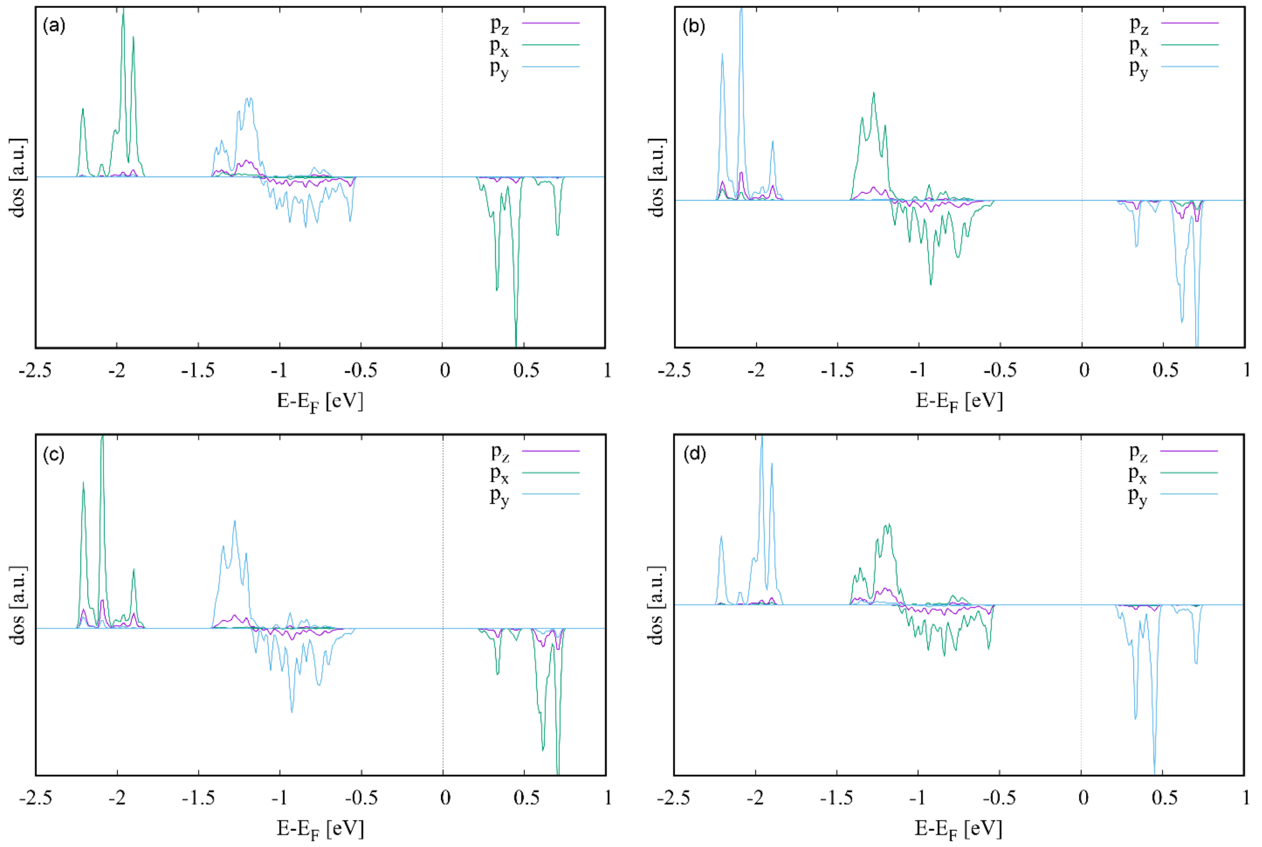


**FIG. S11** Partial density of states (DOS) for selected $O_2^-$ molecules, showing orbital ordering in the $P\bar{4}$ structure. (a) Partial DOS for $O_2^-$ molecules labeled 8 and 9. (b) Partial DOS for $O_2^-$ molecules 5 and 10. (c) Partial DOS for $O_2^-$ molecules 6 and 11. (d) Partial DOS for $O_2^-$ molecules 7 and 12. Atomic labels according to Fig. 1 (c) – (f) in the main text.

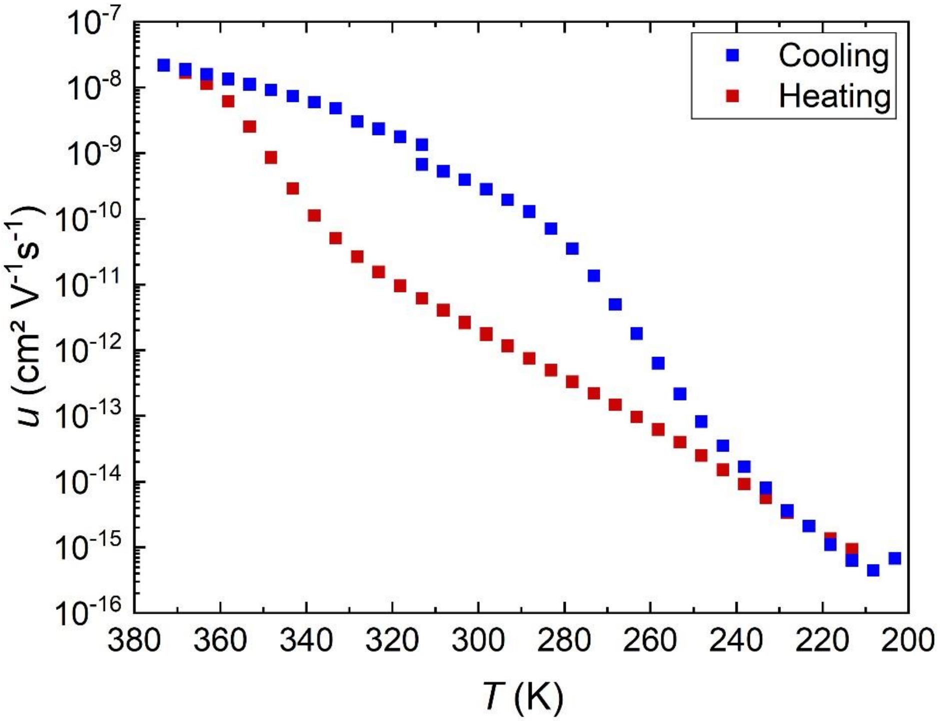


**FIG. S12** Temperature-dependent charge carrier mobility of $Rb_4O_6$. One assumption has been made: The cell volume shows a temperature-dependent expansion or contraction as shown in Fig. 2 of the main text. In the range of the phase transition a linear change of the volume from $V_{cub}$ to $V_{tet}$ and vice versa is assumed.

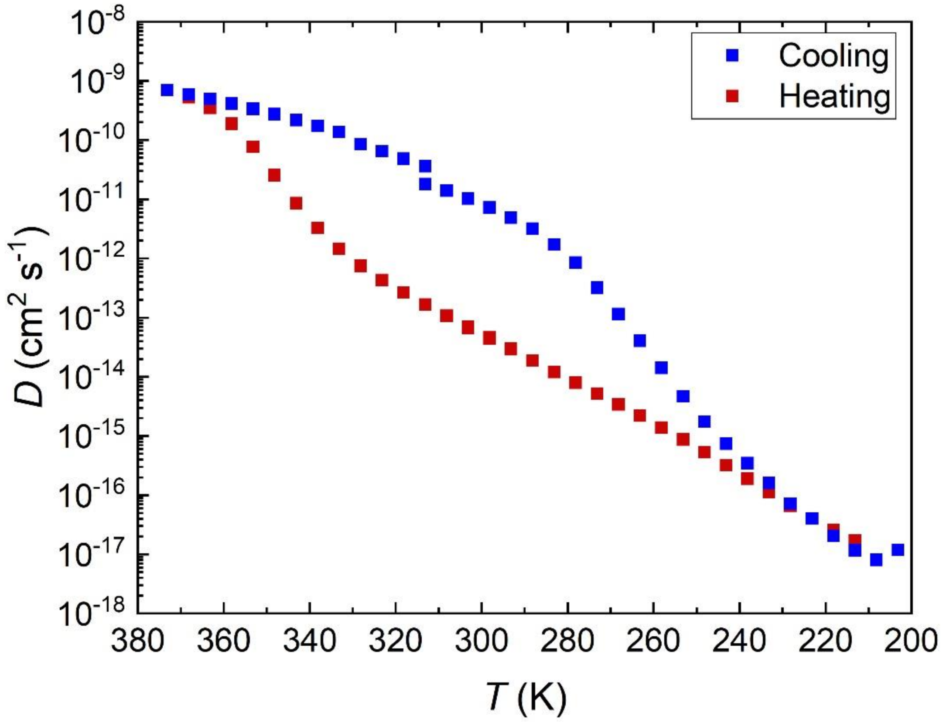


**FIG. S13** Temperature-dependent diffusion coefficients of $Rb_4O_6$. The diffusion coefficient of the electrons in the cubic phase is almost three orders of magnitude higher than the diffusion coefficient of the electrons in the tetragonal phase at the same temperature.

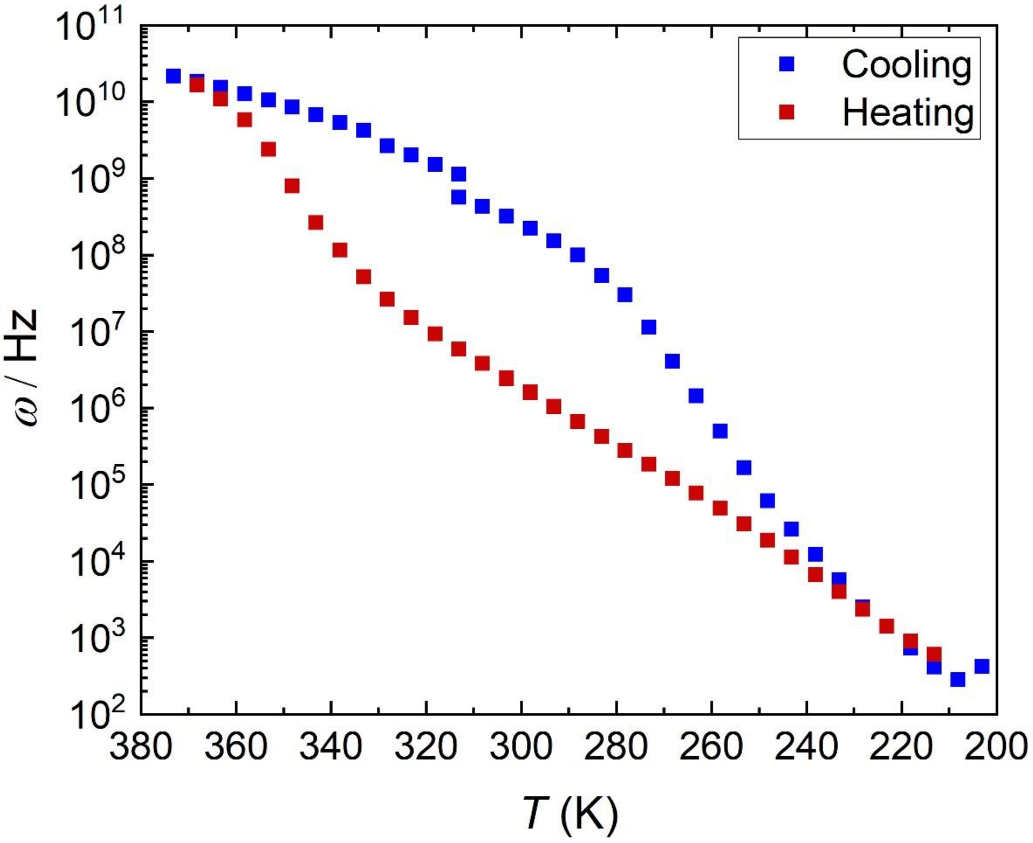


**FIG. S14** Temperature-dependent jump frequency of the electrons in $Rb_4O_6$. Jump distance (distance between the oxygen dumbbells) in the cubic phase: $a$ = 439 pm. Jump distance in the tetragonal phase: $a$ = 418 pm.

**Table S1.** Results of the crystal structure refinements of $Rb_4O_6$ from powder neutron diffraction data measured at instrument E9. The refinement of the cubic crystal structure was carried out in the space group $I\bar{4}3d$ (No. 220), while the two tetragonal structures were refined in $I\bar{4}$ (No. 82) and $P\bar{4}$ (No. 81), respectively. The isotropic temperature factors of the Rb atoms as well as those of the O atoms were constrained to be equal for the tetragonal phase.

| Neutron data of $Rb_4O_6$ at 2.9 K | | | | | |
|---|---|---|---|---|---|
| Atom | Site | *x* | *y* | *z* | *B* [Å] |
| Rb11 | 4*h* | 0.6985(13) | 0.9399(12) | 0.0349(10) | 0.57(5) |
| Rb12 | 4*h* | 0.1944(12) | 0.4539(13) | 0.5533(9) | 0.57 |
| Rb21 | 4*h* | 0.3196(11) | 0.4545(12) | 0.2018(10) | 0.57 |
| Rb22 | 4*h* | 0.7947(11) | 0.9259(10) | 0.7176(9) | 0.57 |
| O11 | 2*e* | 0 | 0 | 0.0738(3) | 0.98(5) |
| O12 | 2*f* | ½ | ½ | 0.5738(3) | 0.98 |
| O21 | 2*g* | 0 | ½ | 0.1752(5) | 0.98 |
| O22 | 2*g* | 0 | ½ | 0.3227(5) | 0.98 |
| O31 | 4*h* | 0.2196(8) | 0.1758(10) | 0.4343(4) | 0.98 |
| O32 | 4*h* | 0.7309(13) | 0.6185(13) | 0.9347(7) | 0.98 |
| O41 | 4*h* | 0.2675(13) | 0.1132(11) | 0.3206(4) | 0.98 |
| O42 | 4*h* | 0.7955(12) | 0.5933(10) | 0.8207(6) | 0.98 |

$a = b = 8.6494(3)$, $c = 10.3473(5)$ Å, $V = 774.10(7)$ Å$^3$, $R_F = 0.041$, $\chi^2 = 3.36$

| Neutron data of $Rb_4O_6$ at 100 K | | | | | |
|---|---|---|---|---|---|
| Atom | Site | *x* | *y* | *z* | *B* [Å] |
| Rb1 | 8*g* | 0.6962(8) | 0.9454(8) | 0.0425(8) | 1.55(4) |
| Rb2 | 8*g* | 0.3093(9) | 0.4471(9) | 0.2067(8) | 1.55 |
| O1 | 4*e* | 0 | 0 | 0.0735(3) | 1.96(5) |
| O2 | 4*f* | 0 | ½ | 0.1765(3) | 1.96 |
| O3 | 8*g* | 0.2197(8) | 0.1014(6) | 0.4312(4) | 1.96 |
| O4 | 8*g* | 0.2681(8) | 0.1397(7) | 0.3156(4) | 1.96 |

$a = b = 8.6700(3)$, $c = 10.3641(4)$ Å, $V = 779.06(6)$ Å$^3$, $R_F = 0.043$, $\chi^2 = 2.86$

| Neutron data of $Rb_4O_6$ at 400 K | | | | | |
|---|---|---|---|---|---|
| Atom | Site | *x* | *y* | *z* | *B* [Å] |
| Rb | 16*c* | 0.94437(18) | 0.94437 | 0.94437 | 6.35(8) |
| O | 24*d* | 0.55304(27) | 0 | ¾ | 7.95(12) |

$a = b = c = 9.3861(5)$ Å, $V = 826.92(15)$ Å$^3$, $R_F = 0.106$, $\chi^2 = 3.72$

**Table S2.** Interatomic distances (in Å) as obtained from the crystal structure refinements of $Rb_4O_6$ powder neutron diffraction data collected at instrument E9. Constraints were used to assure meaningful O-O distances for the superoxide $O_2^-$ and peroxide $O_2^{2-}$ units. Also listed are the tilting angles α and β (in °) of the superoxide $O_2^-$ units relative to the *a* and *c* axes, respectively, obtained at 2.9 and 100 K.

| Bond / Angle | $Rb_4O_6$ at 2.9 K<br>$P\bar{4}$ (No 81) | $Rb_4O_6$ at 100 K<br>$I\bar{4}$ (No 82) | $Rb_4O_6$ at 400 K<br>$I\bar{4}3d$ (No. 220) |
|---|---|---|---|
| *d*(Rb11-O11/O11) | 2.689(11)/2.887(11) | 2.695(7)/2.934(7) | 2.999(3) |
| *d*(Rb12-O12/O12) | 2.682(10)/2.979(10) | 2.695/ 2.934 | |
| *d*(Rb11-O21/O22) | 2.819(11)/4.113(11) | 2.876(8)/4.185(9) | 2.916(2) |
| *d*(Rb12-O22/O21) | 2.945(11)/4.277(11) | 2.876/ 4.185 | |
| *d*(Rb11-O32/O32/O32/O31) | 2.947(16)/2.981(15)/3.299(16)/4.310(12) | 3.030(10)/3.204(9)/3.250(9)/4.114(10) | |
| *d*(Rb12-O31/O31/O31/O32) | 2.711(14)/2.832(15)/3.792(14)/4.048(12) | 3.030/ 3.204/ 3.250/ 4.114 | |
| *d*(Rb11-O42/O41/O42/O42) | 2.881(14)/3.015(12)/3.188(14)/3.822(14) | 2.928(10)/2.941(10)/3.598(9)/3.606(9) | |
| *d*(Rb12-O42/O41/O41/O41) | 2.798(12)/2.903(15)/3.415(14)/ 3.844(14) | 2.928/ 2.941/ 3.598/ 3.606 | |
| *d*(Rb21-O12/O12) | 2.825(11)/4.173(11) | 2.851(9)/4.171(9) | |
| *d*(Rb22-O11/O11) | 2.867(10)/4.141(11) | 2.851/ 4.171 | |
| *d*(Rb21-O21/O22) | 2.806(10)/3.060(10) | 2.739(8)/2.978(8) | |
| *d*(Rb22-O21/O22) | 2.853(10)/2.662(9) | 2.739/ 2.978 | |
| *d*(Rb21-O32/O32/O32/O31) | 2.828(15)/2.868(13)/3.354(15)/3.514(13) | 2.868(10)/2.897(10)/3.248(10)/3.872(10) | |
| *d*(Rb22-O31/O31/O32/O31) | 2.998(13)/3.063(11)/3.524(13)/3.862(13) | 2.868/ 2.897/ 3.248/ 3.872 | |
| *d*(Rb21-O42/O42/O41/O42) | 3.053(15)/3.214(14)/3.243(14)/4.088(13) | 2.828(10)/ 2.916(9)/3.426(10)/4.177(10) | |
| *d*(Rb22-O41/O42/O41/O41) | 3.003(14)/3.069(13)/3.203(14)/4.147(11) | 2.828/ 2.916/ 3.426/ 4.177 | |
| *d*(O11-O11) | 1.527(5) | 1.524(4) | 1.351(4) |
| *d*(O12-O12) | 1.528(5) | 1.524 | 1.351 |
| *d*(O21-O22) | 1.527(7) | 1.525(4) | 1.351 |
| *d*(O31-O41) | 1.336(10) | 1.312(7) | 1.351 |
| α(O31-O41) | 58.8(5) | 38.3(5) | |
| β(O31-O41) | 28.3(5) | 20.1(5) | |
| *d*(O32-O42) | 1.323(11) | 1.312 | 1.351 |
| α(O31-O41) | 21.4(5) | 38.3 | |
| β(O31-O41) | 26.9(5) | 20.1 | |

**Table S3.** The connection between atomic labels (Fig. 6c in the main text and in the Tables S1, S2) and molecule labels (Figs. 1(c)-(f) in the main text) as used in DFT calculations for the crystal structure of $Rb_4O_6$ at 2.9 K ($P\bar{4}$).

| Atomic labels | DFT molecule labels |
|---|---|
| O31 and O41 | 5, 6, 10 and 11 |
| O32 and O42 | 7, 8, 9 and 12 |

**Table S4.** Hopping integrals $t^2$ between nearest neighboring $O_2^-$ molecules as given by DFT calculations for the crystal structure of $Rb_4O_6$ at 100 K ($I\bar{4}$). Labels used are the same as in Figure 1 in the main text.

| Molecule pair | $t^2$ [eV$^2$] | Molecule pair | $t^2$ [eV$^2$] | Molecule pair | $t^2$ [eV$^2$] |
|---|---|---|---|---|---|
| 10 ↔ 5 | 0.378 | 8 ↔ 10 | 0.191 | 8 ↔ 12 | 0.018 |
| 7 ↔ 12 | 0.378 | 11 ↔ 7 | 0.191 | 11 ↔ 5 | 0.018 |
| 9 ↔ 10 | 0.225 | 8 ↔ 7 | 0.191 | 9 ↔ 5 | 0.014 |
| 6 ↔ 7 | 0.225 | 11 ↔ 10 | 0.191 | 6 ↔ 12 | 0.014 |
| 10 ↔ 6 | 0.225 | 8 ↔ 5 | 0.018 | 9 ↔ 12 | 0.014 |
| 9 ↔ 7 | 0.225 | 11 ↔ 12 | 0.018 | 5 ↔ 6 | 0.014 |

**Table S5.** Total energies for two different spin configurations as given by DFT calculations for the crystal structure of $Rb_4O_6$ at 2.9 K ($P\bar{4}$). Labels used are the same as in Figure 1 in the main text.

| Molecule labels | 5 8 | 9 10 | 7 11 | 6 12 | Total energy [eV] |
|---|---|---|---|---|---|
| FM configuration | ↑ ↑ | ↑ ↑ | ↑ ↑ | ↑ ↑ | -65814.477743 |
| AFM configuration | ↑ ↓ | ↑ ↓ | ↑ ↓ | ↑ ↓ | -65814.483039 |
